# Supplementary material for: Generating Phishing Attacks using ChatGPT
Source: arXiv:2305.05133 source file (2023-05-09)
Supplement: Supplementary file 1 [file appendix.tex]

\subsubsection{Computing code similarity between websites}
\label{appendix-code-similarity}
\sayak{Need to somehow include this in main text}
\sayak{Also need to extend this so we can say: phishing attacks on FHDs share similar codebase, they also share similar codebase with legitimate attacks}

Automated anti-phishing tools often assume that benign websites share very little code with phishing attacks. However, in Section~\ref{characterization}, we found that nearly 71.4\% of code is shared between phishing attacks and benign websites hosted on FHD services, which is primarily caused by attackers using the same website templates and design tools as benign websites created on the service. To compute the similarity between two websites, Website A and Website B (sim\textsubscript{A to B}) we first extracted the tags elements of both websites. For a particular tag element T in Website A, the Levenshtein distance is calculated between that tag element and every tag element of Website B, with the tag in Website 2 having the lowest LV distance being selected as the tag with the maximum similarity T\textsubscript{max} for that particular tag in Website A. This is computed for each tag in Website A, and the website similarity between Website A and Website B is the median of all T\textsubscript{max} values. The similarity between Website B and Website A (sim\textsubscript{B to A}) is also computed in the same way. The overall similarity between two websites (sim\textsubscript{A,B}) is computed as the mean of sim\textsubscript{A to B} and sim\textsubscript{B to A}. Table~\ref{table-website-similarity} illustrates the computed median code similarity between phishing and benign URLs of five FHDs, which provide users with a website design template, and five others that do not provide such functionality. Each phishing website for an FHD (Website A) was compared with a benign website from the same FHD (Website B). We find that the FHDs which provide design templates have a much higher code similarity than the FHDs that dont.

\begin{table}[t]
\centering
\begin{tabular}{|l|c|c|}
\hline
FHD & \# URLs & Median similarity \\ \hline
Weebly (T) & 1,307 & 81.2\% \\ 
000webhostapp (T) & 1,096 & 73.8\% \\ 
Blogspot (T) & 689 & 61.7\% \\ 
Google Sites (T) & 541 & 77.4\% \\ 
Wix (T) & 496 & 68.1\% \\ 
DuckDNS (NT) & 1,096 & 16.8\% \\ 
Github.io (NT) & 401 & 23.1\% \\
MyFTP.org (NT) & 191 & 13.7\% \\
Firebase (NT) & 330 & 27.1\% \\ 
Atwebpages (NT) & 145 & 8.2\% \\
\hline
\end{tabular}
\caption{Website code similarity between phishing and benign websites from some popular FHDs. For each FHD, T in parenthesis denotes that the FHD has a design template, and NT denotes that the FHD does not have a design template}
  \label{table-website-similarity}
\end{table}

\subsubsection*{Common phrases in FHD phishing URL strings}
\label{appendix-common-phrases}
One of the features that we utilize for automatically detecting FHD-based phishing attacks in Section~\ref{feature-extraction} is to identify phrases, which are commonly found in the URL strings of FHD-based phishing attacks. To identify these phrases, we tokenized the URL strings of all 8,859 phishing websites in our dataset (D1). The list of the commonly occurring words in these URL strings is illustrated through a Word cloud in Figure~\ref{fig:extension-in-action}. We pick the 30 most commonly occurring words for our feature set.

\begin{figure}[t]
\centering
  \includegraphics[width=0.6\columnwidth]{figures/word_cloud_common_phrases.pdf}
\caption{Wordcloud of the most common phrases found in the URL string of FHD phishing attacks}
  \label{fig:wordcloud}
\end{figure}

\subsubsection*{Cumulative distribution of website takedown time for reported URLs} 
\label{appendix-website-takedown}
In Section~\ref{reporting-fhd-phishing} we identified for new websites reported by FreePhish,  the responsiveness and takedown speed varied across the different FHDs/hosting registrars. The cumulative distribution of the removal time for both reported and non-reported URLs is illustrated in Figure~\ref{fig:reported_cdf}. 

% \begin{figure}[t]
% \centering
%   \includegraphics[width=0.6\columnwidth]{figures/reported_cdf.pdf}
% \caption{Example of an FHD phishing website containing an embedded iFrame for another phishing attack hosted over a traditional domain.}
%   \label{fig:reported_cdf}
% \end{figure}

\subsubsection*{Some examples of FHD phishing attacks}
% At least 16 out of 24 FHDs provide users with templates to build their own website, with most of them providing additional tools to customize the website. However, based on the layouts of the FHD-based phishing attacks in our dataset, we find a disparity in the efforts put in by attackers to design their attacks. Several websites look professional and very closely resemble their targeted organization, such as Fig ~\ref{fig:pro1} and ~\ref{fig:pro2} while others have crude designs~\ref{fig:crude1} or link to It would be interesting to see if users are still susceptible to the latter. 
A few examples of FHD based phishing attacks. While some are well made and closely resemble their targeted organization, such as Figure~\ref{fig:pro1} and ~\ref{fig:pro22}, others have a crude design (Fig ~\ref{fig:crude1}) or use a button to link to an external phishing website~\ref{fig:button_phish}. It would be interesting to explore how users are susceptible to FHD phishing attacks of various complexities. 

\begin{figure}[t]
\centering
  \includegraphics[width=0.6\columnwidth]{figures/pro1.png}
\caption{A phishing website hosted on Wix which closely emulates the login page of Chase. In this case the attacker has obfuscated the website banner.}
  \label{fig:pro1}
\end{figure}
\begin{figure}[h!]
\centering
  \includegraphics[width=0.5\columnwidth]{figures/pro2.png}

\caption{A phishing website hosted on duckdns which closely resembles Netflix.}
  \label{fig:pro22}
\end{figure}
% \begin{figure}[t]
% \centering
%   \includegraphics[width=0.35\columnwidth]{figures/pro3.png}
% \caption{A multi-level phishing attack hosted on Weebly, which asks for your Instagram username before transferring you to an external phishing website.}
%   \label{fig:pro2}
% \end{figure}
\begin{figure}[t]
\centering  
\includegraphics[width=0.5\columnwidth]{figures/crude1}
\caption{A crudely designed phishing attack hosted on Yolasite which imitates the login page for Outlook.com. Here the attacker has not obfuscated the website banner as it is clearly visible at the footer of the website.}
  \label{fig:crude1}
\end{figure}
% \begin{figure}[t]
% \centering
%   \includegraphics[width=0.5\columnwidth]{figures/crude2.png}
% \caption{A crudely designed phishing attack on Weebly which asks for your credentials to access a document. Note how the attacker attempts to obfuscate the credential text by introducing special characters.}
%   \label{fig:crude2}
% \end{figure}
% \begin{figure}[h!]
% \centering
%   \includegraphics[width=0.7\columnwidth]{figures/crude3}

% \caption{A crudely designed login page for Yahoo! on Google Sites. While the attacker has obfuscated the website banner, there was not much effort put into its design.}
%   \label{fig:extension-in-action}
% \end{figure}

% \begin{figure}[h!]
% \centering
%   \includegraphics[width=0.7\columnwidth]{figures/fhd_iframe.pdf}
    
% \caption{Example of an FHD phishing website containing an embedded iFrame for another phishing attack hosted over a traditional domain.}
%   \label{fig:btb-fhd}

% \end{figure}
\begin{figure}[t!]
\centering
  \includegraphics[width=0.9\columnwidth]{figures/button_phish.pdf}
\caption{Example of a two-step phish: The landing page is hoted using FHD which only contains a button only and no credential requiring field, Clicking the button results in the user being directed to an attacker-hosted phishing website with asks for the user's login credentials.}
  \label{fig:button_phish}

\end{figure}
